# Supplementary material for: CLIP4STR: A Simple Baseline for Scene Text Recognition with Pre-trained Vision-Language Model
Source: arXiv:2305.14014 source file (2024-12-24)
Supplement: Supplementary file 4 [file supp-main.tex]

\begin{table}[!t]
    \centering
    \caption{\textbf{Word accuracy on 8 common benchmarks}.
    The\colorbox{Gray1}{best}and\colorbox{Gray2}{second-best}results are highlighted.
    Benchmark datasets~(\textbf{B}) - SVT, IIIT5K, IC13, and IC15.
    `N/A' for not applicable.}
    \setlength\tabcolsep{4pt}
    \scalebox{0.75}{
    \begin{tabular}{l|l|l|cccccccccc}
    \toprule
    \multirow{2}{*}{Method} 
    & \multirow{2}{*}{Pre-train Data}  & \multirow{2}{*}{Train Data}
    & IIIT5K & SVT & IC13 & IC15 & IC15 & SVTP & CUTE & HOST & WOST \\
    &  &  & 3,000 & 647 & 1,015 & 1,811 & 2,077 & 645 & 288 &2,416
    & 2,416\\
    \midrule
    \rowcolor{red!50}
    0-shot CLIP~\cite{2021-clip} & WIT 400M~\cite{2021-clip} & N/A &
    90.0 & -- & -- & -- & -- & -- & -- & -- & -- &\\
    \midrule

    PARSeq$_A$~\cite{2022_parseq} & From Scratch & MJ+ST
    & 97.0 & 93.6 & 96.2 & 86.5 & 82.9 & 88.9 & 92.2 & -- & -- \\

    TrOCR$_{Large}$~\cite{li2021trocr} & Textlines-684M & MJ+ST+B
    & 94.1 & 96.1 
    & 97.3 & 88.1 & 84.1 & 93.0 & 95.1 & -- & --\\

    SIGA$_{T}$~\cite{guan2023self} & ImageNet-1K & MJ+ST
    & 96.6 & 95.1 & 96.8 & 86.6 & 83.0 & 90.5 & 93.1 & -- & -- \\
    \rowcolor{red!50}
    CLIP-OCR~\cite{wang2023symmetrical} & From Scratch & MJ+ST
    & 97.3 & 94.7 & -- & 87.2 & -- & 89.9 & 93.1 & -- & -- \\
    \rowcolor{red!50}
    LISTER-B~\cite{cheng2023lister} & N/A & MJ+ST
    & 96.9 & 93.8 & -- & 87.2 & -- & 87.5 & 93.1 & -- & -- \\
    \rowcolor{red!50}
    CLIPTER~\cite{aberdam2023clipter} & N/A & Real(1.5M)
    & -- & 96.6 & -- & -- & 85.9 & -- & -- & -- & -- \\
    
    DiG-ViT-B~\cite{yang2022reading} & Textimages-33M & Real(2.8M) 
    & 97.6 & 96.5 & 97.6 & 88.9 & -- & 92.9 & 96.5 & 62.8 & 79.7 \\
    \rowcolor{red!50}
    CCD-ViT-B~\cite{guan2023selfccd} & Textimages-33M & Real(2.8M) 
    & 98.0 & 97.8 & 98.3 & 91.6 & -- & 96.1 & 98.3 & -- & -- \\
    
    PARSeq$_A$~\cite{2022_parseq} & From Scratch & Real(3.3M)
    & 99.1 & 97.9 
    & 98.4
    & 90.7 & 89.6 & 95.7 & 98.3 & 74.4 & 85.4 \\

    MAERec-B~\cite{jiang2023revisiting} & Union14M-U & Union14M-L
    & 98.5 & 97.8 
    & 98.1
    & - & 89.5 & 94.4 & 98.6 & - & - \\

    \midrule
    \midrule
    CLIP4STR-B & \multirow{4}{*}{WIT 400M}
    & MJ+ST
    & 97.7 & 95.2 & 96.1 & 87.6 & 84.2 & 91.3 & 95.5
    & 79.8 & 87.0 \\

    CLIP4STR-L & & MJ+ST
    & 98.0 & 95.2 & 96.9 & 87.7 & 84.5 & 93.3 & 95.1 
    & \cellcolor{Gray1}{82.7} 
    & 88.8 \\

    CLIP4STR-B & & Real(3.3M)
    & 99.2 
    & 98.3 
    & 98.3 
    & {91.4}
    & {90.6} 
    & {97.2} 
    & \cellcolor{Gray1}{99.3}
    & 77.5 
    & 87.5 \\

   CLIP4STR-L & & Real(3.3M)
    & \cellcolor{Gray2}{99.5}
    & {98.5}
    & {98.5}
    & 91.3 
    & {90.8} 
    & {97.4} 
    & 99.0
    & 79.8 
    & {89.2} \\

    \hdashline[1pt/1pt]
    CLIP4STR-B &\multirow{3}{*}{DataComp-1B~\cite{gadre2024datacomp}}  & Real(3.3M)
    & 99.4
    & \cellcolor{Gray2}98.6
    & 98.3 
    & 90.8
    & 90.3 
    & 97.8
    & 99.0
    & 77.6 
    & 87.9 \\

    CLIP4STR-B & & RBU(6.5M)
    & \cellcolor{Gray2}99.5
    & 98.3
    & 98.6
    & 91.4
    & 91.1
    & 98.0
    & 99.0
    & 79.3 
    & 88.8 \\

    CLIP4STR-L & & RBU(6.5M)
    & \cellcolor{Gray1}99.6
    & \cellcolor{Gray2}98.6
    & \cellcolor{Gray1}99.0
    & \cellcolor{Gray1}91.9
    & \cellcolor{Gray1}91.4 
    & \cellcolor{Gray1}98.1
    & \cellcolor{Gray1}99.7
    & 81.1 
    & \cellcolor{Gray2}90.6 \\

    CLIP4STR-H & DFN-5B~\cite{fang2023data} & RBU(6.5M)
    & \cellcolor{Gray2}99.5
    & \cellcolor{Gray1}99.1
    & \cellcolor{Gray2}98.9
    & \cellcolor{Gray2}91.7
    & \cellcolor{Gray2}91.0
    & \cellcolor{Gray2}98.0
    & 99.0
    & \cellcolor{Gray2}82.6 
    & \cellcolor{Gray1}90.9 \\

    \bottomrule
  \end{tabular}}
  \label{supp-tab:main-results}
  % \vspace{-1em}
\end{table}
